# Supplementary material for: Low-noise amplification and frequency conversion with a multiport microwave optomechanical device
Source: arXiv:1602.05779 ancillary file (2016-02-18)
Supplement: Supplementary file 1 [file OckeloenKorppi2015_SI.pdf]

# Supplementary information to "Low-noise amplification and frequency conversion with a multiport microwave optomechanical device"

C. F. Ockeloen-Korppi,[1] E. Damskägg,[1] J.-M. Pirkkalainen,[1] T. T. Heikkilä,[2] F. Massel,[2] and M. A. Sillanpää[1]

[1]*Department of Applied Physics, Aalto University, PO Box 11100, FI-00076 Aalto, Finland*
[2]*Department of Physics, Nanoscience Center, University of Jyväskylä, PO Box 35 (YFL), FI-40014 University of Jyväskylä, Finland*

(Dated: February 11, 2016)

## THEORETICAL MODEL

In this section we provide some further details of the theoretical description of the system. In the laboratory frame, the Hamiltonian of the system is given by

$$H = \omega_1 a^\dagger a + \omega_2 c^\dagger c + \omega_m b^\dagger b + \left(g_1 a^\dagger a + g_2 c^\dagger c\right)\left(b^\dagger + b\right) \tag{S1}$$

where $a$ and $c$ represent the cavity modes for cavity 1 and 2 with resonant frequencies $\omega_1$ and $\omega_2$, while $b$ ($b^\dagger$) is the lowering (raising) operator associated with the mechanical resonator, with resonant frequency $\omega_m$. The coupling between the cavities and the mechanics is described in terms of radiation pressure interaction with coupling constants $g_1$ and $g_2$. We follow [1] and consider below the experimental situation where the pump frequencies satisfy $\omega_{P-} = \omega_2 - \omega_m$ and $\omega_{P+} = \omega_1 + \omega_m$. We then expand the cavity operators around the classical response. In the rotating frame with respect to cavity frequencies, the first quantum corrections are described by $H = H_0 + H_I$, where the uncoupled Hamiltonian is $H = \omega_m(b^\dagger b + c^\dagger c - a^\dagger a)$. Retaining only the resonant terms in the remaining linearized interaction yields the coupling Hamiltonian

$$H_I = (G_- c^\dagger + G_+ a)b + h.c., \tag{S2}$$

where $G_- = g_2\sqrt{n_2}$, $G_+ = g_1\sqrt{n_1}$, and $n_2$ and $n_1$ are the photon numbers for the red-detuned and blue-detuned pumping tones for cavity 2 and 1. Applying the two-mode squeezing operator $S(\xi) = \exp\left[\xi c^\dagger a^\dagger - \xi ca\right]$, to the cavity operators

$$\begin{aligned}\eta_{\rm A} &= S^\dagger(\xi) c S(\xi) = \cosh\xi\, c + \sinh\xi\, a^\dagger \\ \eta_{\rm B} &= S^\dagger(\xi) a S(\xi) = \cosh\xi\, a + \sinh\xi\, c^\dagger,\end{aligned} \tag{S3}$$

the Hamiltonian $H_I$ can be recast as a beam-splitter Hamiltonian

$$H_{\rm I} = \mathcal{G}\left(\eta_{\rm A} b^\dagger + \eta_{\rm A}^\dagger b\right), \tag{S4}$$

where we have defined

$$\cosh\xi = G_-/\mathcal{G}, \quad \sinh\xi = G_+/\mathcal{G} \quad \text{with } \mathcal{G}^2 = G_-^2 - G_+^2, \tag{S5}$$

with $G_- > G_+$. Note here how $\eta_{\rm B}$ is a mechanically dark mode (i.e. it does not couple to the mechanics). Assuming the standard dissipation mechanism for the cavities and the mechanics, with dissipation coefficients given by $\kappa$ (equal for both cavities) and $\gamma$, the quantum Langevin equations for $\eta_{\rm A}$ and $\eta_{\rm B}$ can be solved to give [2]

$$\eta_{\rm A} = \frac{\chi_{\rm m}^{-1}}{\chi_{\rm m}^{-1}\chi_{\rm c}^{-1} + \mathcal{G}^2}\sqrt{\kappa}\eta_{\rm A} - \frac{i\mathcal{G}\sqrt{\gamma}}{\chi_{\rm m}^{-1}\chi_{\rm c}^{-1} + \mathcal{G}^2} b_{\rm in} \tag{S6}$$

$$\eta_{\rm B} = \chi_c\sqrt{\kappa}\cosh\xi\, a_{\rm in} + \chi_c{}^*\sqrt{\kappa}\sinh\xi\, c_{\rm in}^\dagger, \tag{S7}$$

where $\chi_{\rm m} = [\gamma/2 - i\omega]^{-1}$ and $\chi_{\rm c} = [\kappa/2 - i\omega]^{-1}$ are the bare mechanical and cavity responses in the rotating frame. Transforming back $\eta_{\rm A}$ and $\eta_{\rm B}$ to $a$ and $c$,

$$\begin{aligned}a &= S(\xi) a S^\dagger(\xi) = \cosh\xi\,\eta_{\rm B} - \sinh\xi\,\eta_{\rm A}^\dagger \\ c &= S(\xi) c S^\dagger(\xi) = \cosh\xi\,\eta_{\rm A} - \sinh\xi\,\eta_{\rm B}^\dagger\end{aligned} \tag{S8}$$

and, taking into account the input-output relations for the cavity fields [3],

$$a_{\rm out} + a_{\rm in} = \sqrt{\kappa_{\rm e}} a$$
$$c_{\rm out} + c_{\rm in} = \sqrt{\kappa_{\rm e}} c, \tag{S9}$$

we can write the expression for the output fields $a$ and $c$. It reads

$$\begin{aligned} a_{\rm out} &= (-\kappa_{\rm e}\mathcal{A}_{aa} - 1)a_{\rm in} - \kappa_{\rm e}\mathcal{A}_{ac}c^\dagger_{\rm in} \\ &\quad - \sqrt{\kappa_{\rm i}\kappa_{\rm e}}\mathcal{A}_{aa}a_{I,\rm in} - \sqrt{\kappa_{\rm i}\kappa_{\rm e}}\mathcal{A}_{ac}c^\dagger_{I,\rm in} + i\sqrt{\gamma\kappa_{\rm e}}\frac{G_+}{(\chi_c\chi_m)^{-1}+\mathcal{G}^2}b^\dagger_{\rm in} \end{aligned} \tag{S10}$$

$$\begin{aligned} c_{\rm out} &= (\kappa_{\rm e}\mathcal{A}_{cc} - 1)c_{\rm in} + \kappa_{\rm e}\mathcal{A}_{ca}a^\dagger_{\rm in} \\ &\quad + \sqrt{\kappa_{\rm i}\kappa_{\rm e}}\mathcal{A}_{cc}c_{I,\rm in} + \sqrt{\kappa_{\rm i}\kappa_{\rm e}}\mathcal{A}_{ca}a^\dagger_{I,\rm in} - i\sqrt{\gamma\kappa_{\rm e}}\frac{G_-}{(\chi_c\chi_m)^{-1}+\mathcal{G}^2}b_{\rm in} \end{aligned} \tag{S11}$$

where

$$\begin{aligned} \mathcal{A}_{aa} &= (\chi^e_c \sinh^2\xi - \chi_c\cosh^2\xi)^* \\ \mathcal{A}_{cc} &= \chi^e_c\cosh^2\xi - \chi_c\sinh^2\xi \\ \mathcal{A}_{ca} = \mathcal{A}^*_{ac} &= (\chi^e_c - \chi_c)\cosh\xi\sinh\xi \end{aligned} \tag{S12}$$

and $\chi^e_c = \chi_{\rm c}\left(1+\mathcal{G}^2\chi_{\rm c}\chi_{\rm m}\right)^{-1}$ represents the effective cavity response in the presence of the two-tone optomechanical drive. In eqs. (S10, S11), we have explicitly included the possibility of internal cavity losses (and noise) for both cavities by introducing the operators $a_{I,\rm in}$ and $c_{I,\rm in}$. From eqs. (S11, S12), one readily obtains the direct gain $A_{\rm d}$ and cross gain $A_{\rm x}$ for output field $a$,

$$\begin{aligned} A_{\rm d} &= -\kappa_{\rm e}\mathcal{A}_{aa} - 1 \\ A_{\rm x} &= -\kappa_{\rm e}\mathcal{A}_{ac}. \end{aligned} \tag{S13}$$

For $G_- \simeq G_+$ (while keeping $G_- \geq G_+$), we can express the maximum gains $A_{\rm d}$ and $A_{\rm x}$ as

$$A_{\rm d}|_{\omega=0} \approx 2\left[\frac{\kappa_e}{\kappa}\frac{4G_-^2/\kappa}{\gamma+4\mathcal{G}^2/\kappa}\right], \quad A_{\rm x}|_{\omega=0} \approx 2\left[\frac{\kappa_e}{\kappa}\frac{4G_-G_+/\kappa}{\gamma+4\mathcal{G}^2/\kappa}\right]. \tag{S14}$$

Moreover, the bandwidth of amplification is given by the effective mechanical damping, given by

$$\gamma_{\rm eff} = \gamma + \frac{4\mathcal{G}^2}{\kappa}. \tag{S15}$$

When the bandwidth is determined by the optomechanical pumping, i.e., $4\mathcal{G}^2/\kappa \gg \gamma$, the expressions for the direct and cross-gains become particular simple,

$$A_{\rm d}|_{\omega=0} \overset{4\mathcal{G}^2\gg\gamma\kappa}{\approx} 2\left[\frac{\kappa_e}{\kappa}\frac{1}{1-x^2}\right], \quad A_{\rm x}|_{\omega=0} \overset{4\mathcal{G}^2\gg\gamma\kappa}{\approx} 2\left[\frac{\kappa_e}{\kappa}\frac{x}{1-x^2}\right], \tag{S16}$$

where $x = G_+/G_- \lesssim 1$.

From the expression of the output fields given by eq. (S10), the added noise at the output port of cavity 1, assuming direct amplification, can be written as

$$\begin{aligned} S_{\rm add,d} &= \frac{1}{2}\langle a^\dagger_{\rm out}a_{\rm out} + a_{\rm out}a^\dagger_{\rm out}\rangle - \frac{1}{2}|A_{\rm d}|^2\langle a^\dagger_{\rm in}a_{\rm in} + a_{\rm in}a^\dagger_{\rm in}\rangle \\ &= \kappa_{\rm i}\kappa_{\rm e}|\mathcal{A}_{aa}|^2\left(n^T_a + \frac{1}{2}\right) \\ &\quad + |\kappa_{\rm e}\mathcal{A}_{ac}|^2\left(n_c + \frac{1}{2}\right) + \kappa_{\rm i}\kappa_{\rm e}|\mathcal{A}_{ac}|^2\left(n^T_c + \frac{1}{2}\right) \\ &\quad + \frac{\gamma\kappa_{\rm e}G_+^2}{|(\chi_c\chi_m)^{-1}+\mathcal{G}^2|^2}\left(n^T_m + \frac{1}{2}\right) \end{aligned} \tag{S17}$$

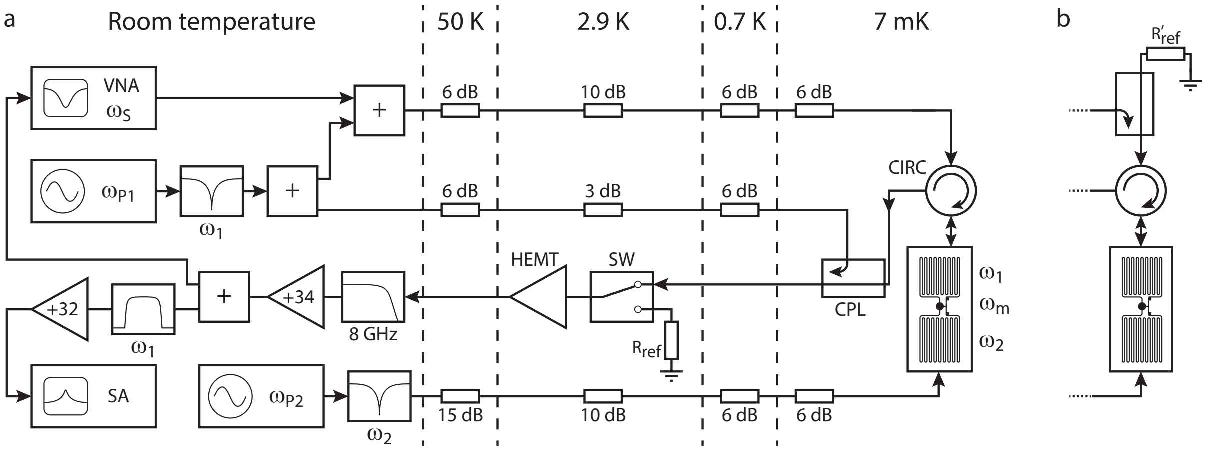


Figure S1. Measurement setup and cryogenic temperature stages. a) Main setup. Shown are network analyzer (VNA), signal generators ($\omega_{\rm P1}$, $\omega_{\rm P1}$), signal analyzer (SA), power splitters / combiners (+), circulators (CIRC), directional coupler (CPL), switch (SW), noise source $\rm R_{ref}$, HEMT amplifier, filters, attenuators and room-temperature amplifiers. b) Alternative low-temperature setup used in a separate calibration cooldown.

while for cross-amplification we have

$$
\begin{aligned}
S_{\rm add,x} &= \frac{1}{2}\langle a^\dagger_{\rm out}a_{\rm out} + a_{\rm out}a^\dagger_{\rm out}\rangle - \frac{1}{2}\left|A_{\rm x}\right|^2 \langle c^\dagger_{\rm in}c_{\rm in} + c_{\rm in}c^\dagger_{\rm in}\rangle \\
&= |-\kappa_{\rm e}\mathcal{A}_{aa} - 1|^2\left(n_a + \frac{1}{2}\right) + \kappa_{\rm i}\kappa_{\rm e}|\mathcal{A}_{aa}|^2\left(n_a^T + \frac{1}{2}\right) \\
&\quad + \kappa_{\rm i}\kappa_{\rm e}|\mathcal{A}_{ac}|^2\left(n_c^T + \frac{1}{2}\right) \\
&\quad + \frac{\gamma\kappa_{\rm e}G_+^2}{|(\chi_c\chi_m)^{-1} + \mathcal{G}^2|^2}\left(n_m^T + \frac{1}{2}\right),
\end{aligned} \tag{S18}
$$

and analogous expressions hold for cavity 2. From eqs. (S18) and (S19) in the large-gain limit ($G_- \simeq G_+$) and for small internal losses ($\kappa_{\rm e} \gg \kappa_{\rm i}, \gamma$), both $S_{\rm add,d}$ and $S_{\rm add,x}$ approach the quantum limit ($S_{\rm add,d}/|A_{\rm d}|^2 \simeq S_{\rm add,x}/|A_{\rm x}|^2 \gtrsim 1/2$).

It is interesting to note how the contribution from the mechanical resonator bath is reduced in this scheme compared to the amplification with only blue-detuned cavity driving [2]. Namely, for a signal on resonance ($\omega = 0$), and for $4\mathcal{G}^2 \gg \kappa\gamma$ the equivalent added noise from the mechanical bath (last lines on Eqs. (S17) and (S18)) is

$$
S_{\rm add,m}/|A_{\rm d}|^2 = \frac{4\gamma\kappa^2G_+^2}{\kappa_e G_-^4}\left(n_m^T + \frac{1}{2}\right). \tag{S19}
$$

For cross-amplification this result is further multiplied by $G_-^2/G_+^2$. These results mean that near-quantum limited amplification is possible even when the bath of the mechanical resonator responsible for the non-linear interaction is not very close to its ground state.

## EXPERIMENTAL SETUP

Our measurement setup is shown in figure S1a. We use a Bluefors dry dilution refrigirator to cool the sample to a base temperature of 7 mK. The input lines are attenuated at each temperature stage to prevent thermal noise from reaching the sample, so that the sample sees essentially only vacuum noise at its inputs.

The two pump tones, here labelled $\omega_{\rm P1}$ and $\omega_{\rm P2}$, are generated by Anritsu MG3692C signal generators, and passed through a notch filter tuned to $\omega_1$ and $\omega_2$, respectively, to prevent generator phase noise from coupling to the cavities, and injected into cavity 1 and 2, respectively. The probe tone at $\omega_s$ is generated by a R&S ZVA40 vector network analyzer (VNA) is combined with either probe $\omega_{\rm P1}$ (shown) or $\omega_{\rm P2}$, depending on the measurement. All signal generators and analyzers are frequency locked to the same reference.

The output signal of cavity 1 is separated from the input by a circulator, and pre-amplified by a HEMT amplifier (LNF-LNC4_8A) at 2.9 K. To avoid saturating the HEMT amplifier, we add part of the pump signal to the sample output using a directional coupler, carefully adjusted to cause negative interference with the pump signal that was reflected off the sample. At the input of the HEMT amplifier, a mechanical switch can switch in a thermal noise source at 2.9 K to give an absolute calibration of the output power (described below).

The output signal is further amplified at room temperature, and split to the input of the VNA and of a Anritsu MS2830A signal analyzer (SA). The SA input signal is first passed through a filter with a pass-band of a few MHz around $\omega_1$, in order to further reduce the amplitude of the pump tone $\omega_{\mathrm{P1}}$.

We also use the VNA to measure the line shape of cavity 1 in a reflection measurement. To establish a reference of the background reflection due to the tranmission lines and filters, we fit a polynomial to the magnitude data outside the cavity resonance. We then devide the complex reflection data by this fit, and extract $\kappa_{\mathrm{int}} = 2\pi \times (0.50 \pm 0.05)$ MHz and $\kappa_{\mathrm{ext}} = 2\pi \times (4.8 \pm 0.2)$ MHz from the resulting amplitude and phase data. The background fit is also used to calibrate the amplifier gain, assuming a gain of 1 (perfect reflection) off resonance from the cavity. For plotting theory curves, we assume cavity 2 to have the same line width as cavity 1.

**Calibration of output noise and system gain**

A precise calibration of the power at the output of the sample is crucial for our measurements. We perform this calibration by comparing to a known noise source $\mathrm{R}_{\mathrm{ref}}$. We first turn off all pump and probe tones and measure the vacuum noise originating from the mK stage. At the signal analyzer (SA), this results in a noise power spectral density (PSD) of $S_0 = (\frac{1}{2} + S_{\mathrm{H}})A_{\mathrm{H}}^2$, expressed in number of quanta (multiplication by $\hbar\omega$ gives power per unit bandwidth). Here, $S_{\mathrm{H}}$ is the effective noise added by the cryogenic HEMT amplifier, and $A_{\mathrm{H}}^2$ is the total power gain from the input of the HEMT to the SA. Then, we flip switch SW and measure the reference noise $S_1 = (S_{\mathrm{ref}} + S_{\mathrm{H}})A_{\mathrm{H}}^2$, where $S_{\mathrm{ref}} = 8.67$ is the thermal noise of resistor $\mathrm{R}_{\mathrm{ref}}$ at a measured temperature of 2.91 K. By comparing these measurements, we find $S_{\mathrm{H}} = 17.6 \pm 1.3$ and $A_{\mathrm{H}}^2 = (75.7 \pm 0.3)$ dB.

In a typical measurement, we wish to measure the output PSD of the sample, $S_{\mathrm{out}}$, which results in $S_{\mathrm{SA}} = (\alpha S_{\mathrm{out}} + S_{\mathrm{H}})A_{\mathrm{H}}^2$ at the SA. Here, $\alpha$ accounts for any attenuation between the sample and the HEMT amplifier. We estimate $\alpha = -1.5 \pm 1.0$ dB based on the low-temperature cabling. In the main text, we plot the effective output PSD,

$$S_{\mathrm{out,eff}} = \frac{S_{\mathrm{SA}}}{\alpha A_{\mathrm{H}}^2}, \tag{S20}$$

which is equal to $S_{\mathrm{out}}$ plus technical noise. In noise measurements we plot the effective input noise PSD, referred to the input of cavity 1,

$$S_{\mathrm{in,eff}} = \frac{S_{\mathrm{SA}}}{\alpha A_{\mathrm{H}}^2 A_{\mathrm{d}}^2}, \tag{S21}$$

where $A_{\mathrm{d}}$ is the direct gain of the mechanical amplifier, measured independently. We emphasize that the quantities (S20, S21) characterize the total system performance, including the added noise of all further amplification stages. The total calibration uncertainty in (S20) and (S21) is 1.0 dB, dominated by the uncertainty in $\alpha$.

The theory curves in figure 2 of the main text include the quantum noise of the input, the predicted added noise of the mechanical amplifier (equation S18), as well as the effective HEMT noise, and is calculated as

$$S_{\mathrm{in,eff}} = \frac{1}{2} + S_{\mathrm{add,d}} + \frac{S_{\mathrm{H,eff}}}{A_{\mathrm{d}}^2}, \tag{S22}$$

where $A_x$ is the the predicted cross gain of the mechanical amplifier and $S_{\mathrm{H,eff}} = S_{\mathrm{H}}/\alpha$ the effective technical noise of the HEMT amplifier as well as any further amplification stages.

To verify the calibration of $\alpha$, we performed a second cooldown where the reference noise source is at the sample input, as shown in figure S1b. The noisy resistor $R'_{\mathrm{ref}}$ is connected to the sample input, and the input signal and pump are combined with it on a -20 dB directional coupler. The noise resistor has an independent heater and temperature sensor, and we vary its temperature to create a calibrated variable noise source $S_{\mathrm{ref}}(T)$. We measure the PSD at the SA, which is epxected to follow

$$S_{\mathrm{SA}}(T) = \left(S_{\mathrm{ref}}(T) A_{\mathrm{d}}^2 + S_{\mathrm{H,eff}}\right) \alpha A_{\mathrm{H}}^2. \tag{S23}$$

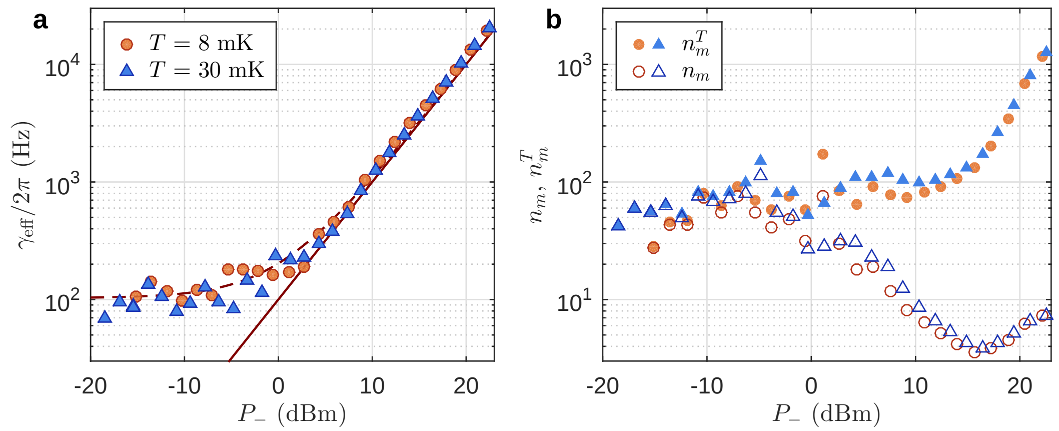


Figure S2. Optomechanical cooling. a) Total linewidth $\gamma_{\rm eff}$ obtained from fits of the output spectrum to equation (S24) at a fridge temperature of 8 mK (circles) and 30 mK (triangles), as a function of pump power. The dashed and solid lines show the fitted $\gamma_{\rm eff}$ and $\gamma_{\rm opt} \propto P_-$, respectively. b) Mechanical mode occupation $n_m$ and mechanical bath temperature $n_m^T$ extracted from the fits, expressed as number of quanta, showing optomechanical cooling down to $n_{m,\rm min} = 3.4$ quanta.

Off cavity resonance ($A_{\rm d}^2 = 1$), a fit to equation (S23) allows us to extract $S_{\rm H,eff}$ independently of $\alpha$ and $A_{\rm H}$. We find $S_{\rm H,eff} = 24$, in excellent agreement with the main calibration described above ($\alpha S_{\rm H} = 25$). With the pumps enabled, and measuring on cavity resonance, equation (S23) also allows us to directly measure the amplifier added noise. However, due to the additional directional coupler in this cooldown the pump power available at the sample was limited to $G_+ \approx G_- \approx 2\pi \times 60$ kHz. At this power, we find $S_{\rm add,d} = 6$ quanta, in good agreement with the values reported figure 3c of the main text.

## Optomechanical cooling

To calibrate the thermal bath temperature of the mechanical oscillator, we perform a series of standard optomechanical cooling measurements. Here, we use a single pump at the lower (red) mechanical side-band co-resonance of cavity 1. The output spectrum at frequency $\delta = (\omega - \omega_1) \ll \kappa, \omega_m$ has a Lorentzian form [4]

$$S_{\rm out}(\delta) = \frac{4\kappa_{\rm e}}{\kappa} n_a^T + \gamma_{\rm opt} \frac{\kappa_{\rm e}}{\kappa} \frac{\gamma_{\rm eff}}{\delta^2 + \gamma_{\rm eff}^2/4} \left(n_m - 2n_a^T\right), \tag{S24}$$

where $\gamma_{\rm eff} = \gamma(T) + \gamma_{\rm opt}$ is the total mechanical line width, $\gamma_{\rm opt}$ the opto-mechanical cooling rate (see eq. (8) in ref. [5]), $n_m$ the occupation of the mechanical mode, and $n_m^T$ and $n_a^T$ the bath temperature of the mechanics and cavity 1, respectively, expressed in number of quanta.

We first calibrate the intrinsic mechanical linewidth $\gamma = 2\pi \times (103 \pm 20)$ Hz from measurements at low pump power and low cryostat temperature $T$, where $\gamma_{\rm eff} \approx \gamma$. Then, we measure the output spectrum as function of pump power $P_-$. We perform the measurements at two temperatures, 8 mK and 30 mK, both in the low-$T$ limit where $\gamma(T) \approx \gamma$. Using the calibrated total system gain from eq. (S20), we can directly fit eq. (S24) to the data and extract the quantities $\gamma_{\rm eff}$, $n_a^T$, and $\gamma_{\rm opt}(n_m - 2n_a^T)$, corresponding to line width, offset and peak area of the Lorentzian, respectively. The fit results show $n_a^T \ll 1$ for all measured powers.

Figure S2a shows the extracted $\gamma_{\rm eff}$ versus $P_-$. Here, the $P_-$ is the output power of the microwave generator. At high powers, $\gamma_{\rm eff}$ is dominated by $\gamma_{\rm opt} \propto P_-$, and we extract the proportionality coefficient from a fit to this data (solid line in figure S2a). Using the now calibrated $\gamma_{\rm opt}$, we caculate $n_m$ from eq. (S24) and $n_m^T$ from the relation [4]

$$n_m^T = \frac{\gamma(T) + \gamma_{\rm opt}}{\gamma(T)} n_m, \tag{S25}$$

which holds for $\gamma_{\rm opt} \ll \kappa \ll 4\omega_m$ and $n_a^T \ll 1$. The results are shown in figure S2. At low pump powers, the mechanical mode is thermalized with the bath. As $P_-$ increases, the mechanical mode is optomechanically cooled, down to $n_{m,\rm min} = 3.4$ quanta. For higher power, cooling is limited by heating of the environment as $n_m^T \propto P_-^2$ up to $n_m^T \approx 10^3$ for the highest pump powers used in our experiments.

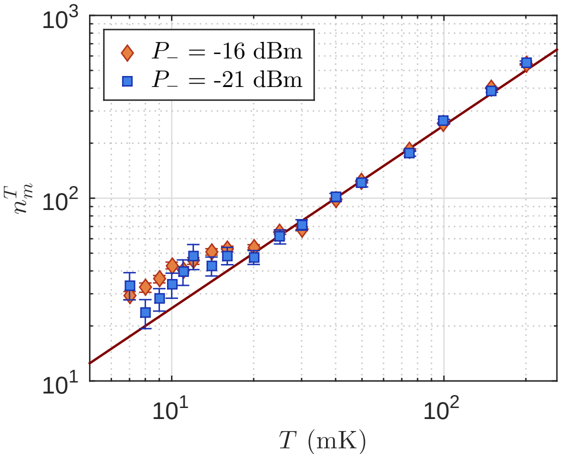


Figure S3. Mechanical oscillator thermalization. Measured mechanical bath temperature $n_m^T$ as a function of cryostat temperature at low cooling power. The mechanical oscillator thermalizes down to 20 mK. The solid line shows the expected thermal occupation. Error bars indicate statistical uncertainty (68% confidence intervals).

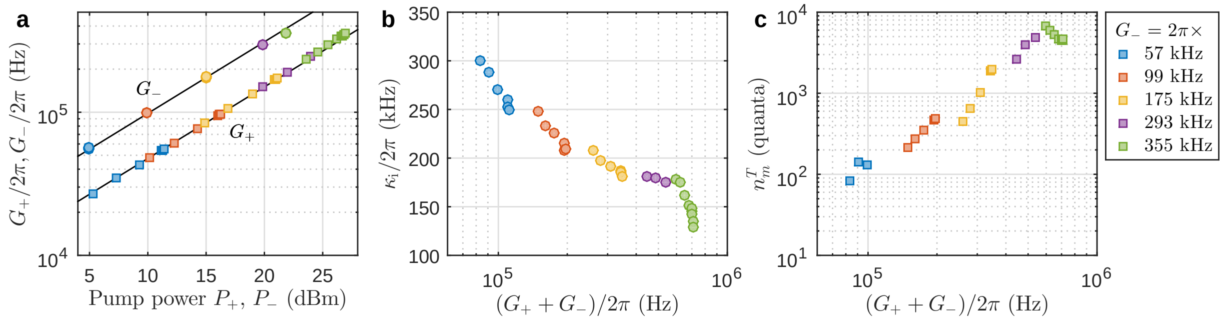


Figure S4. Fit results for two-port amplifier measurements. a) Fitted $G_-$ (circles) and $G_+$ (squares) as function of pump power at the generator. Solid lines show the expected scaling $G_\pm^2 \propto P_\pm$. b) Fitted internal cavity linewidth $\kappa_i$, showing a sharp decrease at the highest pump powers. c) Thermal environment of the mechanical oscillator, expressed as effective number of quanta. In all panels, data with the same color was taken with the same value of $G_-$, as indicated on the legend.

Next, we measure the thermalization between the mechanical bath and the cryostat. We perform again a measurement with a single red-sideband pump, but using low power $P_-$ and varying the temperature of the cryostat. Figure S3 shows $n_m^T$ extracted from fits to eq. (S24), using $\gamma_{\mathrm{opt}}$ calibrated by the data in figure S2a. The data shows that the mechanical mode thermalizes down to 20 mK, showing good agreement with the expected $n_m^T = k_B T/\hbar\omega_m$ (solid line) above this temperature. This agreement also confirms the calibration of the total system gain $\alpha A_{\mathrm{H}}^2$.

## DATA ANALYSIS AND ADDITIONAL DATA

### Two-port amplifier

We measure the direct gain of our amplifier by injecting a weak signal into cavity 1, and recording the resulting reflection spectrum with the VNA. The gain is calibrated by assuming $|A_{\mathrm{d}}|^2 = 1$ outside the cavity resonance. We then record the output noise $S_{\mathrm{out,eff}}$ for the same pump powers but no input signal on the SA, immediately following the gain measurement to avoid any drifts in the gain profile. The input noise $S_{\mathrm{in,eff}} = S_{\mathrm{out,eff}}/|A_{\mathrm{d}}|^2$ is then calculated directly from the data.

To compare our results to theory, we fit the measured direct gain $|A_{\mathrm{d}}|$ to equation (S13) using $G_-$, $G_+$ and $\kappa_{\mathrm{i}}$ as free parameters. In addition, we allow for a $\mathcal{O}$(kHz) frequency shift arising from the radiation pressure force of the pumps. Figure S4a,b shows the results of the fit. We find the coupling strengths $G_\pm^2$ are in excellent agreement with the expected scaling proportional to pump power $P_\pm$. The internal cavity linewidth $\kappa_{\mathrm{i}}$ decreases significantly at high

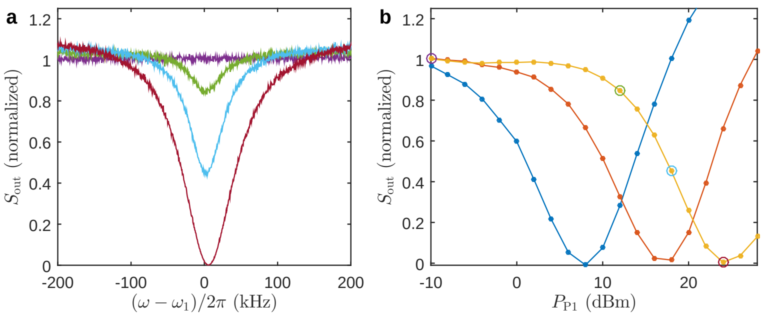


Figure S5. Frequency conversion from cavity 1 to cavity 2. a) Reflection spectrum $S(\omega)$ of cavity 1 (normalized) for $P_{\rm P2}$ = 28 dBm (at the signal generator) and several powers $P_{\rm P1}$, showing a strong dip when the signal is converted to cavity 2. b) Value of $S(\omega)$ at the dip or peak, for a range of pump powers. Circles indicate the data shown in panel a.

pump powers, which is a common effect observed in superconducting circuits and attributed to saturation of two-level systems in the substrate, reducing the effective loss channels.

We then compare our measured noise data $S_{\rm in,eff}$ to the expected theory calculated with equation (S22), where $S_{\rm add}$ is calculated with the parameters obtained from the gain fit. In accordance with the optomechanical cooling measurements discussed in the previous section, we assume $n_a^T = n_c^T \approx 0$, and adjust $n_m^T$. We find that the theory describes the data well for all pump powers with the values for $n_m^T$ shown in figure S4c. The scaling, $n_m^T$ scales approximately with $P_+^2$, and the magnitude is consistent with that observed in figure S2b at high pump powers. At the highest values of $P_+$ the scaling is reduced, which may be related to the steeper decrease in $\kappa_{\rm i}$ observed at those powers (figure S4b).

As discussed in the main text, the amplifier can be tuned within the cavity line width $\kappa$ by shifting the pump frequencies in unison. We find the highest gain is obtained slightly away from the cavity center of the resonance dip observed in reflection measurements. We therefore assume this optimum point to be the true value of $\omega_1$ in the presence of pumping. Similarly, we find the value of $\omega_2$ (which cannot be measured directly in our setup) by maximizing the gain obtained in the two-port amplifier.

## Frequency conversion without amplification

Here we show additional data of frequency conversion without amplification, using the pump scheme depicted in figure 4b in the main text. Figure S5 shows frequency conversion from cavity 1 to cavity 2. The reflected signal of cavity 1 is shown for several pump powers, normalized to unity reflection with all pumps off. As the signal is frequency-converted to cavity 2, a dip is visible in the reflection signal. For balanced pump powers, we observe an attenuation of the signal by 29 dB.

[1] Wang, Y.-D. & Clerk, A. A. Reservoir-engineered entanglement in optomechanical systems. *Phys. Rev. Lett.* **110**, 253601 (2013).
[2] Massel, F. *et al.* Microwave amplification with nanomechanical resonators. *Nature* **480**, 351–354 (2011).
[3] Walls, D. & Milburn, G. J., editors. *Quantum Optics*. Springer-Verlag, Berlin Heidelberg (2008).
[4] Rocheleau, T. *et al.* Preparation and detection of a mechanical resonator near the ground state of motion. *Nature* **463**, 72–75 (2010).
[5] Marquardt, F., Chen, J. P., Clerk, A. A. & Girvin, S. M. Quantum theory of cavity-assisted sideband cooling of mechanical motion. *Phys. Rev. Lett.* **99**, 093902 (2007).
